# Supplementary material for: Sharp Gap-Dependent Variance-Aware Regret Bounds for Tabular MDPs
Source: arXiv:2506.06521 source file (2025-06-06)
Supplement: Supplementary file 1 [file appendix_bak.tex]

\newpage
\appendix

\section{Techinical Lemmas}

\begin{theorem}[Bennett's inequality, Theorem 3 in \citet{maurer2009empirical}]
    \label{thm:bennett}
    Let $X_1,X_2,\cdots,X_n$ be i.i.d. random variables with values $[0,a](a>0)$ and let $\delta>0$. Then, 
    \[\mathbb P\left[\left| \mathbb{E}[X_1] - \frac1n\sum_{i=1}^nX_i \right| > \sqrt{\frac{2\mathbb V[X_1]\log(2/\delta)}{n}} + \frac{a\log(2/\delta)}{n} \right] < \delta. \] 
\end{theorem}

\begin{theorem}[\cite{citation_needed}]
    \label{thm:freedman}
    Let $(X_n)_{n\geq 1}$ be a martingale difference sequence (i.e., $\mathbb E[X_n|\mathcal{F}_{n-1}]=0$ for all $n\geq 1$, where $\mathcal{F}_k=\sigma(X_1,X_2,\cdots,X_k)$) such that $|X_n|\leq a$ for some $a>0$ and for all $n\geq 1$. Let $V_n=\sum_{k=1}^n\mathbb E[X_k^2|\mathcal F_{k-1}]$ for $n\geq 0$. Then, for any positive integer $n$, and any $\varepsilon,\delta>0$, we have \[ \mathbb{P}\left[ \left|\sum_{i=1}^nX_i\right| \geq 2\sqrt{V_n\log(1/\delta)} + 2\sqrt{\varepsilon\log(1/\delta)} + 2a\log(1/\delta)\right] \leq 2(na^2\varepsilon^{-1}+1)\delta.\]
\end{theorem}

We remark that this theorem is given as martingales in many literature. However, this form of martingale differences suits better for this paper.



\section{Validity of estimated upper-bounds}

\begin{lemma}(TBD)
    With probability $1-100SAHK\delta$, for all $(s,a,h,k)\in\State\times\Action\times[H]\times[K]$, \[V_h^k(s)\geq V_h^*(s),Q_h^k(s,a)\geq Q_h^*(s,a)\]
\end{lemma}

\section{Clipping}

This section is dedicated to proving clipping results. The clipped value $\clip{x}{a}$ of $x$ at $a$ is defined as $x\mathbf 1\{x\geq a\}$.

We denote half-clipped values of $E$ as \[\bar{ E}_h^k(x,a)=\clip{{E}_h^k(x,a)}{\frac{\gapmin\Var_h^{*}(x,a)}{2H^2}+\frac{\gapmin}{8H}}.\]

\begin{lemma}
    \[\bar{{V}}_h^k(x)\geq{V}_h^k(x)-\frac{\gapmin}{4}.\]
\end{lemma}

\begin{proof}
    We have $\bar{ E}_h^k(x,a)\geq  E_h^k(x,a)-\frac{\gapmin\Var_h^k(x,a)}{2H^2}-\frac{\gapmin}{2H}$ for any pair of $s,a,h$. Thus, 
    
    \[\begin{aligned}
        &\bar { V}_h^k(x)- V_h^{\pi^k}(x)\\
        =&\mathbb E^{\pi^k}\left[\sum_{h'= h}^H\bar{ E}_h^k(x_h,a_h)\Bigg|x_h=x\right]\\
        \geq&\mathbb E^{\pi^k}\left[\sum_{h'= h}^H{ E}_h^k(x_h,a_h)\Bigg| x_h=x\right]-\frac{\gapmin}{2H^2}\mathbb E^{\pi^k}\left[\sum_{h'=h}^H\mathtt{Var}_h(x_h,a_h)\Bigg| x_h=x\right]-\sum_{h'=h}^H\frac{\gapmin}{8H}\\
        \geq&  V_h^k(x)- V_h^{\pi^k}(x)-\frac{\gapmin}{4},
    \end{aligned}\]

    where the last line is due to Theorem~\ref{thm:Vexpect}.
\end{proof}

This lemma links the half-clipped values $\bar{ V}_h^k$ with the optimal values $ V_h^*$.
\begin{lemma}
    For any pair state-action pair $(s,a)\in S\times A$,
    \[{V}_h^*(x) - {V}_h^{\pi^k}(x,a) \leq 2(\bar{{V}}_h^k(x,a)-{V}_h^{\pi^k}(x)).\]
    %%% The constant is probably wrong.
\end{lemma}

\begin{proof}
    TBA
\end{proof}

This lemma establishes the bound of $\bar{{V}}_h^k(x)-{V}_h^{\pi^k}(x)$.

\begin{lemma}
    Let $\check{E}_h^k(s,a)=\clip{\bar{ E}_h^k(s,a)}{\frac{\Delta_h(s,a)\Var_h^*(s,a)}{3\mathcal V}+\frac{\Delta_h(s,a)}{8H}}$. Then, for any $(s,h)\in \State\times[H]$ and $a=\pi_h^k(s)$, we have \[\bar{{V}}_h^k(s)-{V}_h^{\pi^k}(s) \leq \check{{E}}_h^k(s,a)+\left(1+\frac{\Var_h^*(s,a)}{\mathcal V}+\frac 1{2H}\right)\mathbb{E}^{s'\sim P_{x,a,h}}[\bar{ V}_{h+1}^k(s)- V_{h+1}^{\pi^k}(s)]\]
\end{lemma}

\begin{proof}
    By definition, \[\bar V_h^k(s)-V_h^{\pi^k}(s)=\bar{{E}}_h^k(s,a)+\mathbb{E}^{s'\sim P_{x,a,h}}[\bar{ V}_{h+1}^k(s)- V_{h+1}^{\pi^k}(s)].\]
    Let $a^*=\arg\max_{a'}Q_h^*(s,a')$ be the optimal action. Then, \[Q_h^k(s,a)\geq Q_h^k(s,a^*)\geq Q_h^*(s,a^*)\geq V_h^*(s),\] hence 
    \begin{align}
        \Delta_h(s,a) &= V_h^*(s)-Q_h^*(s,a) \leq Q_h^k(s,a)-r_h(s,a)-\mathbb E^{s'\sim P_{s,a,h}}[V_{h+1}^*(s)] \\
        & = E_h^k(s,a)+\mathbb E^{s'\sim P_{s,a,h}}[V_{h+1}^k(s)-V_{h+1}^*(s)] \\
        & \leq \bar E_h^k(s,a)+\frac{\gapmin\Var_h^*(s,a)}{2H^2}+\frac{\gapmin}{8H}+\mathbb E^{s'\sim P_{s,a,h}}[\bar V_{h+1}^k(s)-V_{h+1}^*(s)]+\frac14\gapmin \\
        & \leq \bar E_h^k(s,a)+\mathbb E^{s'\sim P_{s,a,h}}[\bar V_{h+1}^k(s)-V_{h+1}^*(s)]+\frac12\Delta_h(s,a).
    \end{align}

    We may only consider the case where $\bar{E}_h^k(s,a)<\frac{\Delta_h(s,a)\Var_h^*(s,a)}{3\mathcal V}+\frac{\Delta_h(s,a)}{8H}$. Under this assumption, \[\mathbb E^{s'\sim P_{s,a,h}}[\bar V_{h+1}^k(s,a)-V_{h+1}^*(s,a)]\geq\frac12\Delta_h(s,a)-\frac{\Delta_h(s,a)\Var_h^*(s,a)}{3\mathcal V}-\frac{\Delta_h(s,a)}{8H},\] so, \begin{align*}\bar{E}_h^k(s,a) &\leq \left(\frac{\Var_h^*(s,a)}{3\mathcal V}+\frac{1}{8H}\right)\left(\frac12-\frac{\Var_h^*(s,a)}{3\mathcal V}-\frac1{8H}\right)^{-1}\mathbb E^{s'\sim P_{s,a,h}}[\bar V_{h+1}^k(s)-V_{h+1}^*(s)] \\
    & \leq \left(\frac{\Var_h^*(s,a)}{\mathcal V}+\frac 1{2H}\right)\mathbb E^{s'\sim P_{s,a,h}}[\bar V_{h+1}^k(s)-V_{h+1}^*(s)],\end{align*}

    where the last line is because $\Var_h^*(s,a)\leq \frac14 H^2\leq\frac
    1{200\log 2}\mathcal V.$ and $\frac 12-\frac{\Var_h^*(s,a)}{3\mathcal V}-\frac1{8H}\geq\frac12-\frac{1}{600\log 2}-\frac18>\frac13$.
\end{proof}

We recursively apply this lemma and get \[\bar{{V}}_h^k(s)-{V}_h^{\pi^k}(s) \leq \mathbb E^{\pi^k}\left[\sum_{h'=h}^H\check E_{h'}^k(s_{h'},a_{h'})\prod_{t=h}^{h'-1}\left(1+\frac{\Var_t^k(s_t,a_t)}{\mathcal V}+\frac1{2H}\right)\Bigg| s_h=s\right],\] and hence 

\begin{align}
    \bar V_0^k-V_0^{\pi^k} &\leq \mathbb E^{\pi^k}\left[\sum_{h=1}^H\check E_{h}^k(s_{h},a_{h})\prod_{t=1}^{h-1}\left(1+\frac{\Var_t^k(s_t,a_t)}{\mathcal V}+\frac{1}{2H}\right)\right]\\
    & \leq \mathbb E^{\pi^k}\left[\sum_{h=1}^H\check E_{h}^k(s_{h},a_{h})\prod_{t=1}^{H}\left(1+\frac{\Var_t^k(s_t,a_t)}{\mathcal V}+\frac1{2H}\right)\right] \\
    & \leq \mathbb E^{\pi^k}\left[\sum_{h=1}^H\check E_{h}^k(s_{h},a_{h})\exp\left(\frac12+\sum_{t=1}^{H}\frac{\Var_t^k(s_t,a_t)}{\mathcal V}\right)\right].
\end{align}

By \Cref{thm:Vtail}, \[\mathbb E^{\pi^k}\left[\exp\left(\sum_{t=1}^{H}\frac{\Var_t^k(s_t,a_t)}{\mathcal V}\right) \mathbf 1\left\{\exp\left(\sum_{t=1}^{H}\frac{\Var_t^k(s_t,a_t)}{\mathcal V}\right) \geq \mathrm e\right\}\right] \leq \frac{10}{K\log (K)},\] so \[\bar V_0^k-V_0^{\pi^k}\leq \mathrm e^{3/2}\mathbb E^{\pi^k}\left[\sum_{h=1}^H\check E_{h}^k(s_{h},a_{h})\right] + \frac{10H^2}{K\log (K)}.\] (If $X,Y$ are nonnegative random variables $X,Y$ where $X\leq M$ a.s. for some constant $M$, then for any constant $C$, $\mathbb E[XY]\leq C\mathbb E[X]+M\mathbb E[Y\mathbf 1\{Y\leq C\}]$)

\section{Concentration equalities}

\begin{lemma}
    With probability $1-100SAH\delta$, the following inequalities hold for all $s,a,h$:

    \[|\hat r_h^k(s,a)-r_h(s,a)|\leq\sqrt{\frac{2\mathbb V r_h(s,a)\iota}{n_h^k(s,a)}}+\frac{H\iota}{n_h^k(s,a)},\]
    
    \[|\hat \sigma_h^k(s,a)-\mathbb E[r_h(s,a)^2]|\leq\sqrt{\frac{H^4\iota}{2n_h^k(s,a)}}+\frac{H^2\iota}{n_h^k(s,a)},\]
    
    \[|\langle\hat P_{s,a,h}^k-P_{s,a,h},V_h^*\rangle|\leq\sqrt{\frac{2\mathbb V_{P_{s,a,h}}V_h^*\iota}{n_h^k(s,a)}}+\frac{H\iota}{n_h^k(s,a)},\]
    
    \[|\langle\hat P_{s,a,h}^k-P_{s,a,h},(V_h^*)^2\rangle|\leq\sqrt{\frac{H^4\iota}{2n_h^k(s,a)}}+\frac{H^2\iota}{n_h^k(s,a)},\]
\end{lemma}

\begin{proof}
    By Theorem~\ref{thm:bennett}, Theorem~\ref{thm:freedman}, and union bound.
\end{proof}

\begin{lemma}
    With probability $1-100SAH\delta$, the following inequalities hold for all $s,a,h$:
    \[\left|\sqrt{\hat\sigma_h^k(s,a)-\hat r_h^k(s.a)}-\sqrt{\mathbb V[r_h(s,a)]}\right|\leq \sqrt{\frac{4H^2\iota}{n_h^k(s,a)}},n_h^k(s,a)\geq 2\]
\end{lemma}


\begin{proof}
    \cite{Kevin}'s paper provides a reference for it.
\end{proof}

\section{Estimating Surpluses}

This section is devoted to proving an upper bound of $E_h^k(s_h^k,a_h^k)$.

First, we will assume that value update is $\Trigger$ during the $(k-1)$-th episode. This means \[Q_h^k(s,a)=\hat r_h^k(s,a)+\mathbb E^{s'\sim \hat P_{s,a,h}}[V_{h+1}^k(s')]+b_h^k(s,a).\] Thus,\begin{align}
    E_h^k(s_h^k,a_h^k)&=Q_h^k(s_h^k,a_h^k)-R_h(s_h^k,a_h^k)-\mathbb E^{s'\sim P_{s,a,h}}[V_{h+1}^k(s')]\\
    &=\hat r_h^k(s_h^k,a_h^k)-R_h(s_h^k,a_h^k)+\mathbb E^{s'\sim \hat P{s,a,h}}[V_{h+1}^k(s')]-\mathbb E^{s'\sim P_{s,a,h}}[V_{h+1}^k(s')]+b_h^k(s_h^k,a_h^k)\\
    &\leq C_1\sqrt{\frac{\mathbb Vr_h(s,a)\iota}{n_h^k(s,a)}}+\frac{C_2H\iota}{n_h^k(s,a)} + \mathbb E^{s'\sim \hat P_{s,a,h}^k}[V_{h+1}^k(s')]-\mathbb E^{s'\sim P_{s,a,h}}[V_{h+1}^k(s')]\\
    &\leq .
\end{align}

\section{Closing variance differences}
\begin{align}
    b_h^k(s,a) =& c_1\sqrt{\frac{\mathbb V^{s'\sim \hat P_{s,a,h}}[V_{h+1}^k(s')]\iota}{n_h^k(s,a)}}+c_2\sqrt{\frac{(\hat\sigma_h^k(s,a)-(\hat r_h^k(s,a))^2)\iota}{n_h^k(s,a)}}+c_3\frac{H\iota}{n_h^k(s,a)}\\
    \leq & c_1\sqrt{\frac{\mathbb V^{s'\sim P_{s,a,h}}[V_{h+1}^*(s')]\iota}{n_h^k(s,a)}}+c_1\sqrt{\frac{\mathbb V^{s'\sim P_{s,a,h}}[V_{h+1}^k(s')-V_{h+1}^*(s')]\iota}{n_h^k(s,a)}} \\
     &+c_2\sqrt{\frac{\mathbb V[r_h^k(s,a)]}{n_h^k(s,a)}} +\left|\sqrt{(\hat\sigma_h^k(s,a)-(\hat r_h^k(s,a))^2)}-\sqrt{\mathbb V[r_h^k(s,a)]}\right|\sqrt{\frac{\iota}{n_h^k(s,a)}}\\
    \leq & c_1\sqrt{\frac{\mathbb V^{s'\sim P_{s,a,h}}[V_{h+1}^*(s')]\iota}{n_h^k(s,a)}}+c_2\sqrt{\frac{\mathbb V[r_h(s,a)]\iota}{n_h^k(s,a)}} +\frac{2c_2H\iota}{n_h^k(s,a)} \\
    &+\frac{c_1}{2}\frac{\mathbb V^{s'\sim P_{s,a,h}}[V_{h+1}^k(s')-V_{h+1}^*(s')]}H+ \frac{(c_1/2+c_3)H\iota}{n_h^k(s,a)} \\
    \leq &\sqrt{c_1^2+c_2^2}\sqrt{\frac{\Var_h^k(s,a)\iota}{n_h^k(s,a)}} +\frac{c_1}{2}\frac{\mathbb V^{s'\sim P_{s,a,h}}[V_{h+1}^k(s')-V_{h+1}^{\pi^k}(s')]}H+\frac{(c_1/2+2c_2+c_3)H\iota}{n_h^k(s,a)}
\end{align}
\begin{lemma}
    For any $(s,h,k)\in\State\times[H]\times[K]$, let $h=\pi_h^k(s)$, then
    \begin{align}
    V_h^k(s)-V_h^{\pi^k}(s)=&\hat r_h^k(s,a)+\mathbb E^{s'\sim \hat P_{s,a,h}}[V_{h+1}^k(s')]+b_h^k(s,a)-R_h(s,a)-\mathbb E^{s'\sim \hat P_{s,a,h}}[V_{h+1}^{\pi^k}(s')] \\
     \leq&\sqrt{\frac{2\mathbb V R_h(s,a)\iota}{n_h^k(s,a)}}+\big|\mathbb E^{s'\sim \hat P_{s,a,h}}[V_{h+1}^k(s')-V_{h+1}^*(s')]-\mathbb E^{s'\sim P_{s,a,h}}[V_{h+1}^k(s')-V_{h+1}^*(s')]\big | \\
     & +\big|\mathbb E^{s'\sim P_{s,a,h}}[V_{h+1}^*(s')]-\mathbb E^{s'\sim P_{s,a,h}}[V_{h+1}^*(s')]\big|+|\mathbb E^{s'\sim P_{s,a,h}}[V_{h+1}^k(s')-V_{h+1}^{\pi^k}(s')]|
     \end{align}
\end{lemma}

\section{Putting everything together}
We need the following lemma of sum of clippings:

\begin{lemma}{Lemma B.5, \cite{Kevin}}
    Let $a_1,a_2,\cdots,a_m\geq 0$ be any sequence of nonnegative real numbers. Then $\clip{\sum_{i=1}^ma_i}{\varepsilon}\leq 2\sum_{i=1}^m \clip{a_i}{\varepsilon/2m}$.
\end{lemma}

\begin{corollary}
    Let $\varepsilon_h^k(s,a)=\max\{\frac{\gapmin \Var_h^k(s,a)}{H^2},\frac{\Delta_h(s,a)\Var_h^k(s,a)}{3\mathcal V}\}$. Then, 
    \begin{align}
    \check E_h(s,a)& \leq2\clip{\sqrt{\frac{\mathbb Vr_h(s,a)\iota}{n_h^k(s,a)}}}{\frac{\varepsilon_h(s,a)}{8}} + 2\clip{\frac{C_2H\iota}{n_h^k(s,a)}}{\frac{\varepsilon_h(s,a)}{8}} \\\ 
    & + 2\clip{}{\frac{\varepsilon_h(s,a)}{8}}\mathbb E^{s'\sim\hat P_{s,a,h}}\left[\clip{V_{h+1}^k(s')}{\frac{\varepsilon_h(s,a)}{8}}\right]
    \end{align}
\end{corollary}

%%%% The following parts need to be reviewed


\subsection{Vari}
Notation: $\mathtt{Var}_h^k(x,a)=\mathbb V r_h(x,a)+\mathbb V_{P_{s,a,h}}V_{h+1}^{\pi^k}$.

In another paper, it is proved that \[W^k=\sum_{h=1}^H\mathtt{Var}^{\pi^k}_h(x_h,a_h)\leq 50H^2\iota.\]

Also, the expectation of $W^k$ is bounded by $\frac14 H^2$.

\subsection{Gap between estimated and real variances}

For $X=V_h^k$\todorzout{Again, additional $\sqrt{S}$ factor.} or $X=V_h^*$,

\[\begin{aligned}
    &|\mathbb V_{\hat P_{s,a,h}^k}X-\mathbb V_{P_{s,a,h}^k}X|\leq 
|\langle \hat P_{s,a,h}^k,X^2\rangle-\langle P_{s,a,h},X^2\rangle|+|\langle \hat P_{s,a,h}^k,X\rangle^2-\langle P_{s,a,h},X\rangle^2|\\
\leq & \sqrt\frac{H^4\iota}{2n_h^k(s,a)}+\frac{H^2\iota}{n_h^k(s,a)}+2H\left(\sqrt{\frac{H^2\iota}{2n_h^k(s,a)}}+\frac{H\iota}{n_h^k(s,a)}\right).
\end{aligned}\]

Also, \[\begin{aligned}
    &|\hat \sigma_h^k(x,a)-(\hat r_h^k(s,a))^2-\mathbb Vr_h(x,a)|]\leq|\hat\sigma _h^k(x,a)-(\mathbb Er_h(x,a))^2|+|(\hat r_h^k(s,a))^2-r_h(x,a)^2|\\
    \leq &\sqrt\frac{H^4\iota}{2n_h^k(s,a)}+\frac{H^2\iota}{n_h^k(s,a)}+2H\left(\sqrt{\frac{H^2\iota}{2n_h^k(s,a)}}+\frac{H\iota}{n_h^k(s,a)}\right).
\end{aligned}\]

So, \[b_h^k(s,a)\leq c_1\sqrt{\frac{\mathbb V_{P_{s,a,h}}V_{h+1}^k\iota}{n_h^k(s,a)}}+c_2\sqrt{\frac{\mathbb V r_h(s,a)\iota}{n_h^k(s,a)}}+\frac{c_3H\iota}{n_h^k(s,a)}+\frac{3(c_1+c_2)H^2\iota}{\sqrt 2n_h^k(s,a)}+3(c_1+c_2)H^2\left(\frac{\iota}{n_k^h(s,a)}\right)^{3/2}.\]

(We used for any $x,y,w>0$,$|\sqrt {xw}-\sqrt {yw}|\leq\sqrt{|x-y|w}\leq\frac12(|x-y|+w)$.)

\subsection{Gap between estimated values and real values}
Let $t(k)$ be the last update time before $k$. That is, $t(k)=\arg\max_{k'\leq k}\text{TRIGGERED at the $(k'-1)$-th episode}$. For any $s,a,h$, we have $n_h^{t(k)}(x,a)\geq\frac12 n_h^k(x,a)$ For $a=\pi^k(x)$,\[\begin{aligned}V_h^k(x)-V_h^{\pi^k}(x)&=Q_h^{t(k)}(x,a)-Q_h^{\pi^k}(x,a)\\
&\leq \hat r_h^{t(k)}(x,a)+\langle \hat P_{s,a,h}^{t(k)},V_{h+1}^{t(k)}\rangle+b_h^{t(k)}(s,a)-r_h(x,a)-\langle P_{s,a,h},V^*\rangle\\
&\leq \sqrt\frac{2\mathbb Vr_h(x,a)\iota}{n_h^{t(k)}(s,a)}+\sqrt\frac{2\mathbb V_{P_{s,a,h}}V_{h+1}^{t(k)}\iota}{n_h^{t(k)}(s,a)}+\frac{2H\iota}{n_h^{t(k)}(s,a)}+\langle P_{s,a,h},V_{h+1}^{t(k)}-V_{h+1}^*\rangle+b_h^{t(k)}(s,a).
\end{aligned}\]

Note that $V_h^k(s,a)=V_h^{t(k)}(s,a)$ for any $s,a,h$. Solving recursion yields \[V_h^k(x)-V_h^*(x)\leq\mathbb E^{\pi^k}\left[\sum_{h'\geq h}\\\sqrt\frac{4\mathbb Vr_h(x,a)\iota}{n_h^k(s,a)}+\sqrt\frac{4\mathbb V_{P_{s,a,h}}V_{h+1}^k\iota}{n_h^k(s,a)}+\frac{4H\iota}{n_h^k(s,a)}+b_h^{t(k)}(s,a)\Bigg |x_{h}=x\right].\]



% Following Kevin's paper (no modifications here), we have \[\Delta_h(x,a)\leq E_{k,h}(x,a)+p_h(x,a)^\top(\overline{ V}_{h+1}- V_{h+1}^{\pi^k}),\]\[\bar{ V}_h^{\pi^k}(x)- V_h^{\pi^k}(x)=\bar{ E}_{k,h}(x,\pi_{k,h}(x))+p(x,\pi_{k,h}(x))^\top(\bar{ V}_{h+1}^{\pi^k}- V_{h+1}^{\pi^k}),\] and the half-clipped values are related by the following lemma:

% \[\bar{ E}_{k,h}(x,a)\geq E_{k,h}(x,a)-\varepsilon_{clip},\overline{ V}_{k,h}(x)-\bar{ V}_{k,h}^{\pi^k}(x)\leq (H-h+1)\varepsilon_{clip}.\]

% Denote $\mathbb I(x,a)$ as the event that the trajectory following $\pi^k$ visits the state action pair $(x,a)$ and $\mathbb I(x)$ similarly. Unfolding the recursion, we have, for any $x$, \[\bar { V}_h^{\pi^k}(x)- V_h^{\pi^k}(x)=\mathbb E^{\pi^k}\left[\left.\sum_{h'\geq h}\bar { E}_{k,h'}(x_{h'},\pi_{k,h'}(x_{h'}))\right|\mathbb I(x)\right].\] 

% At the mean time, \[\Delta_h(x,a)\leq \bar{ E}_{k,h}(x,a)+p_h(x,a)^\top(\bar{ V}_{h+1}- V_{h+1}^{\pi^k})+\frac12\Delta_h(x,a),\] and thus, for any $x$, \[\Delta_h(x,\pi_{k,h}(x))\leq 2(\bar { V}_h^{\pi^k}(x)- V_h^{\pi^k}(x)).\]

% Now we compute the following quantity: 

% $$
% \begin{aligned}
%     &\mathbb E^{\pi^k}\left[\sum_{h=1}^H\mathtt{Var}_h^{\pi^k}(x_h,a_h)\Delta_h(x_h,a_h)\right]\\
%     \leq&2\sum_{h=1}^H\sum_x\mathbb E^{\pi^k}\left[\mathbb I(x)\mathtt{Var}_h^{\pi^k}(x,\pi_{k,h}(x))(\bar{ V}_h^{\pi^k}(x)- V_h^{\pi^k}(x))\right]\\
%     =&2\sum_{h=1}^H\sum_x\mathbb E^{\pi^k}\left[\mathbb I(x)\mathtt{Var}_h^{\pi^k}(x,\pi_{k,h}(x))\sum_{h'\geq h}\bar{ E}_{k,h'}(x_{h'},\pi_{x,h'}(x_{h'}))\right]\\
%     =&2\mathbb E^{\pi^k}\left[\sum_{h=1}^H\sum_{h'=h}^H\mathtt {Var}_h^{\pi^k}(x_h,a_h)\bar{ E}_{k,h'}(x_{h'},\pi_{x,h'}(x_{h'}))\right]\\
%     \leq&2\mathbb E^{\pi^k}\left[\sum_{h=1}^H\mathtt {Var}_h^{\pi^k}(x,\pi_{k,h}(x))\sum_{h'=1}^H\bar{ E}_{k,h'}(x_{h'},\pi_{x,h'}(x_{h'}))\right]\\
%     \leq& 2H^2(\bar { V}_0^{\pi^k}- V_0^{\pi^k}).
% \end{aligned}$$

% (We probably need Bernstein inequality to prove that $\mathbb P(\sum_{i=1}^H\mathtt {Var}_h^{\pi^k}(x,\pi_{k,h}(x))>(\log H)^{100}H^2)<H^{-1}$ for the last step, which is yet to be fully verified.)

% The next step involves summing the inequality over $k$. This yields \[\sum_{k=1}^K\sum_{h=1}^H\bar{ E}_{k,h}(x_{k,h},a_{k,h})=\sum_{k=1}^K(\bar{ V}_0^{\pi^k}- V_0^{\pi^k})\geq\frac 1{2H^2}\mathbb E\left[\sum_{k=1}^K\sum_{h=1}^H\mathtt {Var}_h^{\pi^k}(x_{k,h},a_{k,h})\Delta_h(x_{k,h},a_{k,h})\right].\]

% Note that \[\mathtt {Var}_h^*(x,a)-\mathtt {Var}_h^{\pi^k}(x,a)\leq\|\overline{ V}_h(x,a)-\underline { V}_h(x,a)\|_{2,p_h}^2\leq \mathbb E^{\pi^k}\left[\left.100\sum_{h'=h}^H B_c^{fut}(x_{h'},a_{h'})\right|\mathbb I(x,a)\right].\]

% (By Lemma F.8)

% Using the relation, we reorder the terms by $(x,a,h)$ pairs:

% \[\sum_{x,a,h}\min\{\sqrt{\mathtt {Var}_h^*(x,a)n_h(x,a)\iota},\mathtt {Var}_h^*(x,a)\varepsilon_{clip}^{-1}\iota\}+\sum_{x,a,h}H^4S\iota\geq\frac 1{2H^2}\mathbb E\left[\sum_{s,a,h}(\mathtt {Var}_h^*(x,a)\Delta_h(x,a)n_h(x,a)-100SH^4\Delta_h(x,a)\iota)\right]\]

% (By Lemma B.4 and some other calculations, this step requires further verification).

% If the LHS is $\tilde R$, then it is an upper bound of regret. Multiply both sides by $\sum_{(x,a,h)\in\mathcal Z_{sub}}\frac{1}{\Delta_h(x,a)}$ We have, by Cauchy-Schwatz,

% \[\begin{aligned}
%     &\left(\tilde R-\sum_{(x,a,h)\in\mathcal Z_{opt}}\mathtt {Var}_h^*(x,a)\varepsilon_{clip}^{-1}-S^2H^4A\right)\sum_{(x,a,h)\in\mathcal Z_{sub}}\frac{1}{\Delta_h(x,a)}\\
%     \geq &\frac{1}{2H^2}\mathbb E\left[\left(\tilde R-\sum_{(x,a,h)\in\mathcal Z_{opt}}\mathtt {Var}_h^*(x,a)\varepsilon_{clip}^{-1}-S^2H^4A\right)^2\right]-50SH^2\sum_{s,a,h}\Delta_h(x,a)\sum_{s,a,h}\frac{1}{\Delta_h(x,a)},
% \end{aligned}\]

% and all the remaining job is to solve the quadratic, which yields \[R=\tilde O\left(\sum_{(x,a,h)\in\mathcal Z_{sub}}\frac{H^2}{\Delta_h(x,a)}+\frac{|\mathcal Z_{opt}|H^3}{\Delta_{min}}+S^2H^4A\right).\]

% --------------------------------

% \section{What I can do}

% Bernstein style bound of $$\sum_{i=1}^t\alpha_t^i[r_{j,h}(s,a_h^{k_i})+V_{j,h+1}^{k^i}(s_{h+1}^{k^i})]$$.

% The bound is \[\sqrt{\sum_{i=1}^t(\alpha_t^i)^2[\mathbb V_h(r_{j,h}+V_{j,h+1}^{k^i})](s,a)}\]

% The variance can be estimated using all previous values with error $O(poly(S,A)\cdot K^{-1/2})$ (proof to be completed later; similar to Lemma C.7 in the Q-learning paper; also use FTRL theory to close the distribution discrepancy gap).

% Variance law similar to Lemma C.5. (May also contain discrepancies of order $O(poly(S,A)\cdot K^{-1/2})$ from bootstrapping.)=

% \section{Problems to be solved}

% \subsection{FTRL analysis}
% I can only decompose the FTRL error into second-order momentum, instead of variance, plus small terms. If nothing else happens, the total regret will be $\Omega(\sqrt{SH^4\min(A,H)K})$ unless this gap can be closed.

% Possibly we can manipulate the expectation by subtracting a constant.

% (But why does the expectation affect the FTRL regret?)
